# Supplementary material for: Search for the decay $B_s^0 \to \overline{D}^{0} f_{0}(980)$
Source: arXiv:1505.01654 ancillary file (2015-08-07)
Supplement: Supplementary file 1 [file LHCb-PAPER-2015-012-supplementary.pdf]

# 7 Supplementary material

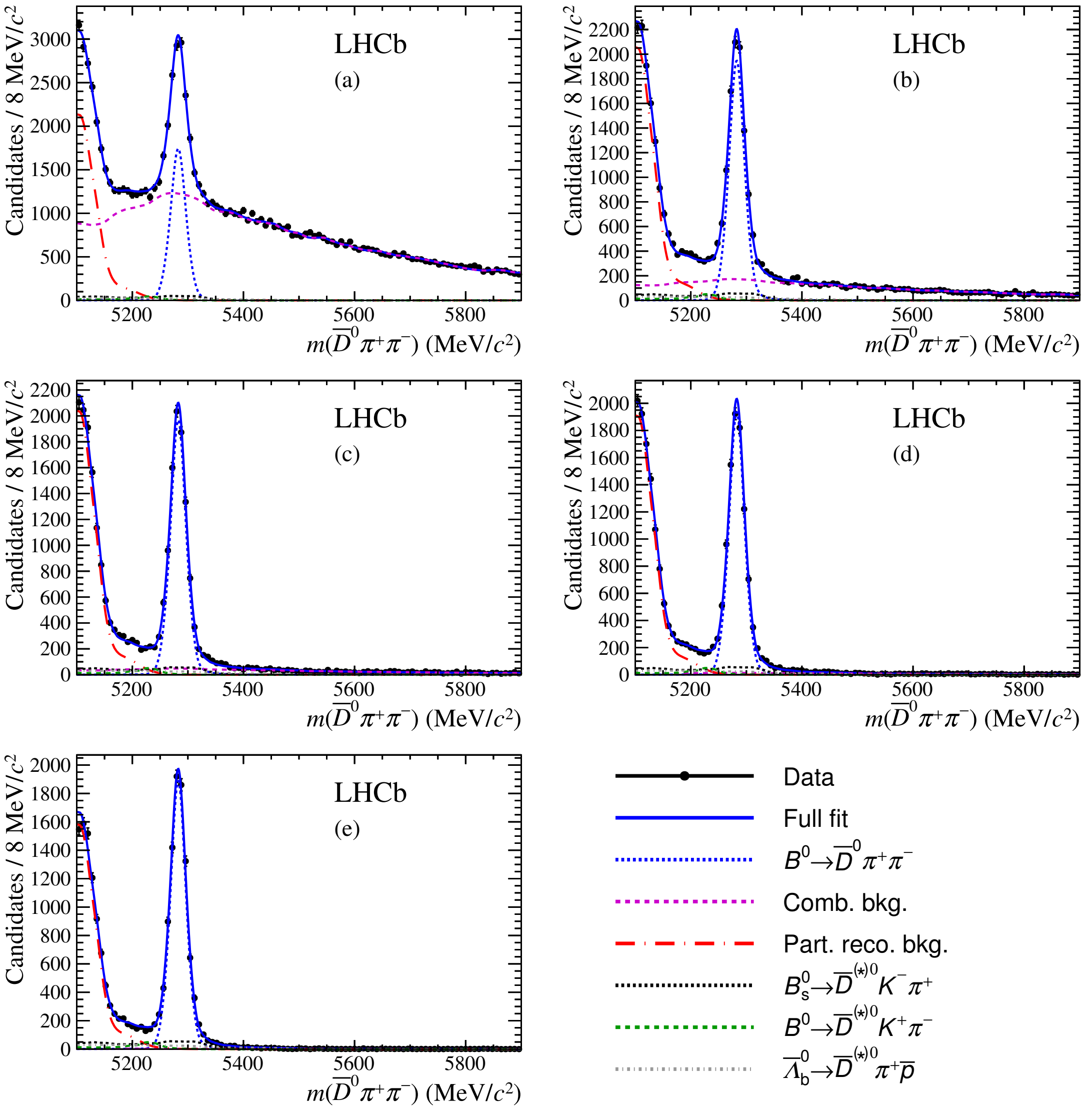


Figure 3: Results of the fits to the $B^0 \to \overline{D}^0\pi^+\pi^-$ data sample. The components are as detailed in the legend. The labels (a) to (e) show the NN bins with increasing purity.

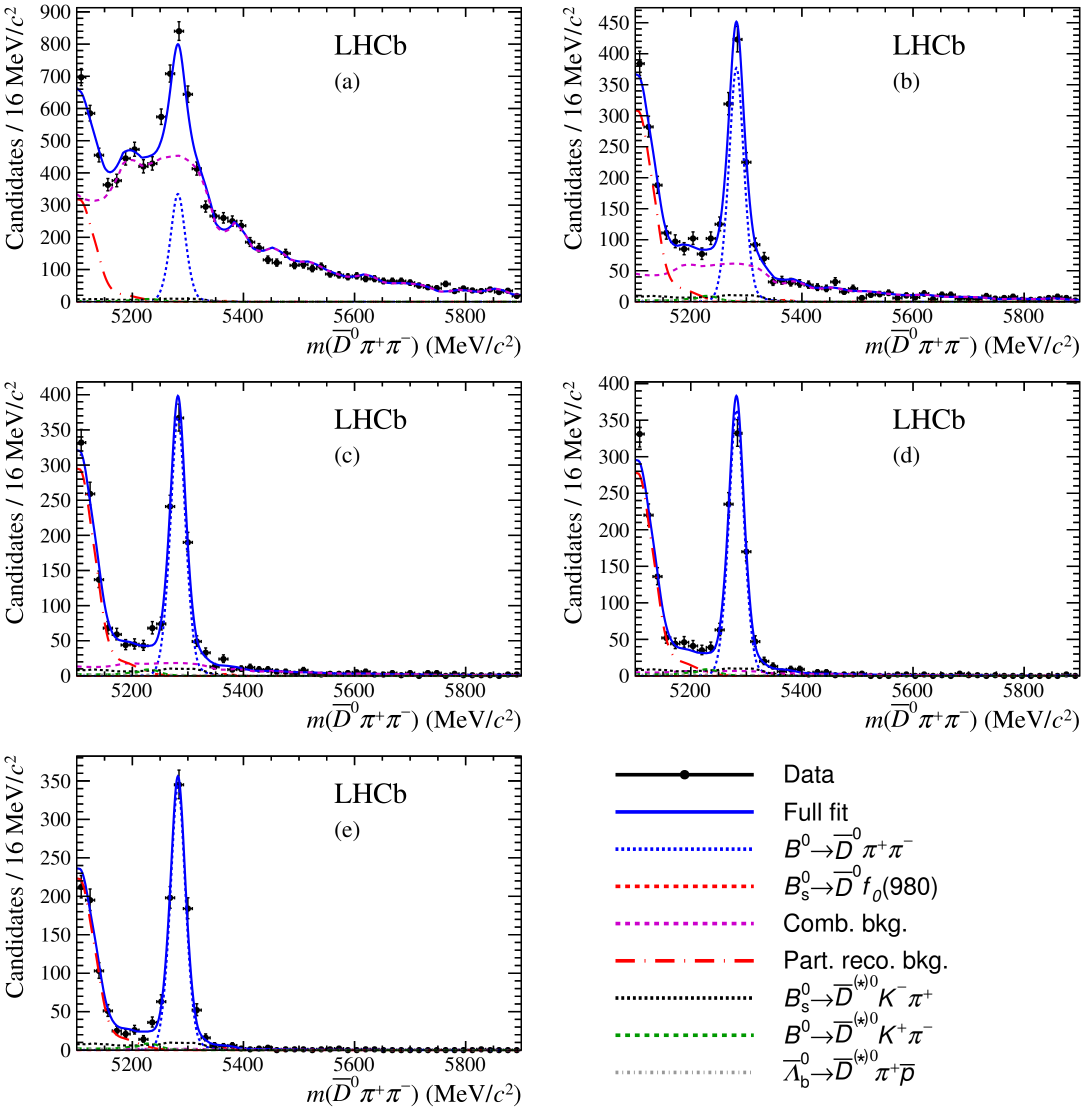


Figure 4: Results of the fits to the $B_s^0 \to \overline{D}^0 f_0(980)$ data sample. The components are as detailed in the legend. The labels (a) to (e) show the NN bins with increasing purity.

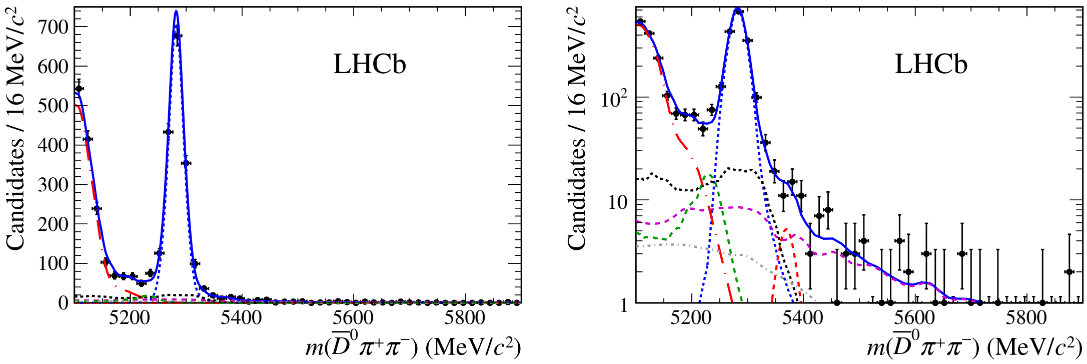


Figure 5: Invariant mass distribution of candidates in the $\overline{D}^0 f_0(980)$ sample with fit results overlaid, in the two highest purity NN output bins shown with (left) linear and (right) logarithmic scales. The solid blue line shows the total fit result and the dashed blue (red) line shows the $B^0$ ($B_s^0$) signal component. The other components are shown as indicated in the legend in Fig. 3.
